# Supplementary material for: Frequency Effects on Syntactic Rule Learning in Transformers
Source: arXiv:2109.07020 source file (2021-09-14)
Supplement: Supplementary file 2 [file acquisition_figure.tex]

\newcommand{\titleboxnatural}[0]{\efbox[backgroundcolor=white]{\transparent{1.0}\footnotesize Natural Sentences}}
\newcommand{\titleboxnonce}[0]{\efbox[backgroundcolor=white]{\transparent{1.0}\footnotesize Nonce Sentences}}
\begin{figure}[ht]
(a)\begin{tikzpicture}
    \pgfplotsset{footnotesize,samples=10}
    \begin{groupplot}[
        group style = {group size = 2 by 1, horizontal sep = 5pt}, 
        width = 4.5cm, 
        height = 4.0cm]
        \nextgroupplot[
            title = {\titleboxnatural},
	        title style={yshift=-6mm},
            ylabel={Error Rate (\%)},
            xmode=log,
            xmin=8, xmax=5500,
            ymin=-5, ymax=80,
            xtick={10, 100, 1000, 10000},
            xticklabels={,,},
            ytick={0, 20, 40, 60},
            ymajorgrids=true,
            xmajorgrids=true,
            grid style=dashed,
            x label style={at={(axis description cs:0.5,-0.2)},anchor=north},
            y label style={at={(axis description cs:-0.125,0.5)},anchor=south},
            ]
            \addplot[
                color=teal,
                mark=diamond,
                mark size=2.5pt,
                ]
                coordinates {
                (10,    37.8)
                (20,    35.6)
                (30,    34.4)
                (40,    21.1)
                (60,    20)
                (80,    14.4)
                (100,   17.8)
                (300,   11.1)
                (1000,  7.8)
                (2000,  7.8)
                (4000,  8.9)
                };
            \addplot[
                color=brown,
                mark=square,
                mark size=1.7pt,
                ]
                coordinates {
                (10,    39.6)
                (20,    33.2)
                (30,    20.4)
                (40,    13.4)
                (60,    9.3)
                (80,    6.3)
                (100,   6.3)
                (300,   4.2)
                (1000,  2.6)
                (2000,  2.5)
                (4000,  2.3)
                };  
        \nextgroupplot[
            title = {\titleboxnonce},
	        title style={yshift=-6mm},
            legend style={at={(-0.0, 1.03)}, anchor=south},
            xmode=log,
            xmin=8, xmax=5500,
            ymin=-5, ymax=80,
            xtick={10, 100, 1000, 10000},
            ytick={0, 20, 40, 60},
            yticklabels={,,},
            ymajorgrids=true,
            xmajorgrids=true,
            grid style=dashed,
            xticklabels={,,},
            legend style={inner sep=0pt},
            x label style={at={(axis description cs:0.5,-0.2)},anchor=north},
            y label style={at={(axis description cs:-0.125,0.5)},anchor=south},
            ]
            \addplot[
                color=teal,
                mark=diamond,
                mark size=2.5pt,
                ]
                coordinates {
                (10,    50.7)
                (20,    50.4)
                (30,    45.6)
                (40,    36)
                (60,    27.3)
                (80,    22.7)
                (100,   21.7)
                (300,   19.7)
                (1000,  18.3)
                (2000,  17)
                (4000,  17.6)
                };
                \addlegendentry{Novel subject-verb pairs}
            \addplot[
                color=brown,
                mark=square,
                mark size=1.7pt,
                ]
                coordinates {
                (10,    41.9)
                (20,    41.8)
                (30,    34.3)
                (40,    25.5)
                (60,    17.6)
                (80,    13.9)
                (100,   14.3)
                (300,   14)
                (1000,  11.2)
                (2000,  12.2)
                (4000,  13.4)
                };  
                \addlegendentry{Common subject-verb pairs}
    \end{groupplot}
\end{tikzpicture}
(b)\begin{tikzpicture}
    \pgfplotsset{footnotesize,samples=10}
    \begin{groupplot}[
        group style = {group size = 2 by 1, horizontal sep = 5pt}, 
        width = 4.5cm, 
        height = 4.0cm]
        \nextgroupplot[
            title = {\titleboxnatural},
	        title style={yshift=-6mm},
            legend style={at={(1.05, 0.7)},anchor=west},
            ylabel={Error Rate (\%)},
            xmode=log,
            xmin=8, xmax=5500,
            ymin=-5, ymax=80,
            xtick={10, 100, 1000, 10000},
            ytick={0, 20, 40, 60},
            ymajorgrids=true,
            xmajorgrids=true,
            xticklabels={,,},
            grid style=dashed,
            x label style={at={(axis description cs:0.5,-0.2)},anchor=north},
            y label style={at={(axis description cs:-0.125,0.5)},anchor=south},
            ]
            \addplot[
                color=violet,
                mark=diamond,
                mark size=2.5pt,
                ]
                coordinates {
                (10,    48)
                (20,    53.4)
                (30,    42.6)
                (40,    29.1)
                (60,    19.3)
                (80,    13.7)
                (100,   12.7)
                (300,   6.8)
                (1000,  5.1)
                (2000,  5.3)
                (4000,  4.2)
                };
            \addplot[
                color=orange,
                mark=square,
                mark size=1.7pt,
                ]
                coordinates {
                (10,    39.9)
                (20,    30.4)
                (30,    17)
                (40,    10.4)
                (60,    7.6)
                (80,    5.1)
                (100,   5.1)
                (300,   3.3)
                (1000,  2)
                (2000,  1.9)
                (4000,  1.7)
                };  
        \nextgroupplot[
            title = {\titleboxnonce},
	        title style={yshift=-6mm},
            legend style={at={(-0.0, 1.03)}, anchor=south},
            xmode=log,
            xmin=8, xmax=5500,
            ymin=-5, ymax=80,
            xtick={10, 100, 1000, 10000},
            ytick={0, 20, 40, 60},
            yticklabels={,,},
            ymajorgrids=true,
            xmajorgrids=true,
            xticklabels={,,},
            grid style=dashed,
            legend style={inner sep=0pt},
            x label style={at={(axis description cs:0.5,-0.2)},anchor=north},
            y label style={at={(axis description cs:-0.125,0.5)},anchor=south},
            ]
            \addplot[
                color=violet,
                mark=diamond,
                mark size=2.5pt,
                ]
                coordinates {
                (10,    50)
                (20,    48.8)
                (30,    43.9)
                (40,    33)
                (60,    26.1)
                (80,    20.6)
                (100,   19.8)
                (300,   18.1)
                (1000,  15.5)
                (2000,  15.8)
                (4000,  16)
                };
                \addlegendentry{Less frequent verb stems}
            \addplot[
                color=orange,
                mark=square,
                mark size=1.7pt,
                ]
                coordinates {
                (10,    50.4)
                (20,    49)
                (30,    43.1)
                (40,    34.3)
                (60,    24)
                (80,    22.1)
                (100,   21.7)
                (300,   20.7)
                (1000,  19.1)
                (2000,  18.5)
                (4000,  19.3)
                };  
                \addlegendentry{More frequent verb stems}
    \end{groupplot}
\end{tikzpicture}
(c)\begin{tikzpicture}
    \pgfplotsset{footnotesize,samples=10}
    \begin{groupplot}[
        group style = {group size = 2 by 1, horizontal sep = 5pt}, 
        width = 4.5cm, 
        height = 4.0cm]
        \nextgroupplot[
            title = {\titleboxnatural},
	        title style={yshift=-6mm},
            legend style={at={(-0.1, 1.03)}, anchor=south},
            xlabel={Training Steps},
            ylabel={Error Rate (\%)},
            xmode=log,
            xmin=8000, xmax=5500000,
            ymin=-5, ymax=100,
            xtick={10000, 100000, 1000000, 10000000},
            ytick={0, 20, 40, 60, 80},
            ymajorgrids=true,
            xmajorgrids=true,
            grid style=dashed,
            x label style={at={(axis description cs:0.5,-0.2)},anchor=north},
            y label style={at={(axis description cs:-0.125,0.5)},anchor=south},
            ]
            \addplot[
                color=blue,
                mark=diamond,
                mark size=2.5pt,
                ]
                coordinates {
                (10000,    64.1)
                (20000,    58.7)
                (30000,    39.5)
                (40000,    26.8)
                (60000,    19.8)
                (80000,    15.4)
                (100000,   15.3)
                (300000,   9.1)
                (1000000,  6.1)
                (2000000,  5.7)
                (4000000,  5.6)
                };
            \addplot[
                color=olive,
                mark=square,
                mark size=1.7pt,
                ]
                coordinates {
                (10000,    31.2)
                (20000,    31.9)
                (30000,    24.6)
                (40000,    16.2)
                (60000,    9.4)
                (80000,    5.8)
                (100000,   5.4)
                (300000,   3.3)
                (1000000,  2.3)
                (2000000,  2.3)
                (4000000,  1.8)
                };  
        \nextgroupplot[
            title = {\titleboxnonce},
	        title style={yshift=-6mm},
            legend style={at={(-0, 1.03)}, anchor=south},
            xlabel={Training Steps},
            xmode=log,
            xmin=8, xmax=5500,
            ymin=-5, ymax=100,
            xtick={10, 100, 1000, 10000},
            ytick={0, 20, 40, 60, 80},
            yticklabels={,,},
            ymajorgrids=true,
            xmajorgrids=true,
            grid style=dashed,
            legend style={inner sep=0pt},
            x label style={at={(axis description cs:0.5,-0.2)},anchor=north},
            y label style={at={(axis description cs:-0.125,0.5)},anchor=south},
            ]
            \addplot[
                color=blue,
                mark=diamond,
                mark size=2.5pt,
                ]
                coordinates {
                (10,    76.1)
                (20,    60.4)
                (30,    54)
                (40,    42.7)
                (60,    35.5)
                (80,    30.9)
                (100,   28.7)
                (300,   24.5)
                (1000,  24.5)
                (2000,  23.4)
                (4000,  23.5)
                };
                \addlegendentry{Incorrect inflection more frequent}
            \addplot[
                color=olive,
                mark=square,
                mark size=1.7pt,
                ]
                coordinates {
                (10,    24.2)
                (20,    37.7)
                (30,    32.8)
                (40,    24.6)
                (60,    15.2)
                (80,    10.9)
                (100,   11.9)
                (300,   12.4)
                (1000,  9.1)
                (2000,  8.6)
                (4000,  10.2)
                };  
                \addlegendentry{Correct inflection more frequent}
    \end{groupplot}
\end{tikzpicture}
\caption{
BERT's error rate on natural and nonce stimuli for varying number of training steps. 
In (a), common subject-verb pairs had frequency >1000 in the training set, and novel subject-verb pairs had frequency zero. 
In (b) less-frequent verb stems occurred <100k times in the training set and more-frequent verb stems occurred >1M times in the training set. 
}
\label{fig:acquisition_figure}
\end{figure}
